# Supplementary material for: CTVIS: Consistent Training for Online Video Instance Segmentation
Source: arXiv:2307.12616 source file (2023-07-24)
Supplement: Supplementary file 1 [file 12_appendix.tex]

\appendix
\label{sec:appendix}

In this appendix, we first briefly describe the source code files. (Appendix~\ref{app:code}). Then we provide the procedure for generating the pseudo-video dataset and the information about the dataset (Appendix~\ref{app:pseudo}). 
In addition, we give more results on VIS (Appendix~\ref{app:vis}). Finally, we extend CTVIS to video panoptic segmentation (Appendix~\ref{app:vps}).

\section{Code}
\label{app:code}
We include the source code in the zip file. Further implementation details of consistent training can be found in \texttt{ct\_plugin.py}, and the training and inference procedures are included in \texttt{ctvis\_model.py}. \texttt{get\_pseudo\_data.py} is used to generate the pseudo-video datasets. Furthermore, all codes, environmental guidelines, model weights and training logs  will be made publicly available.

\section{Pseudo-Video Datasets}
\label{app:pseudo}

\begin{table}[htbp]
  \centering
    \begin{tabular}{l|cc|cc}
    \toprule
    \multirow{2}[2]{*}{Attributions} & \multicolumn{2}{c|}{YTVIS21*} & \multicolumn{2}{c}{OVIS*} \\
                & Train       & Test        & Train       & Test \\
    \midrule
    Images / Videos & 88,462       & 421         & 86,080       & 140 \\
    Instances   & 434,159      & 986         & 405,866      & 881 \\
    Masks       & 434,159      & 29,297       & 405,866      & 73,027 \\
    \bottomrule
    \end{tabular}%
  \caption{The attributions of YTVIS21$^*$ and OVIS$^*$.}
  \label{tab:pseudo}%
\end{table}%

As mentioned in Section~\ref{sec:exp_pseudo}, we adopt the overlapping categories of COCO and VIS datasets for training. 
Specifically, we use COCO to generate pseudo-videos as the training set and select a portion of the target VIS dataset as the validation set. Since the validation set of the VIS dataset used for evaluation is not publicly available, we split the original training set into two non-overlapping parts, respectively used as training and validation sets. 
In order to facilitate reproducibility, we provide a detailed description of the dataset in this appendix. 
For YTVIS22$^*$, we select \textit{person}, \textit{motorbike}, \textit{car}, \textit{airplane}, \textit{train}, \textit{truck}, \textit{boat}, \textit{bird}, \textit{cat}, \textit{dog}, \textit{horse}, \textit{cow}, \textit{elephant}, \textit{bear}, \textit{zebra}, \textit{giraffe}, \textit{flying disc}, \textit{snowboard}, \textit{skateboard}, \textit{surfboard} and \textit{tennis racket} as the categories. 
For OVIS$^*$, we select \textit{person}, \textit{bicycle}, \textit{vehicle}, \textit{motorcycle}, \textit{airplane}, \textit{boat}, \textit{cat}, \textit{dog}, \textit{horse}, \textit{sheep}, \textit{cow}, \textit{elephant}, \textit{bear}, \textit{zebra} and \textit{giraffe} as the categories. 
Specifically, we select only those images and videos from the COCO and target VIS datasets that contain instances of the categories of interest. 
We select 421 and 140 videos from the training set of YTVIS21 and OVIS as the validation of YTVIS$^*$ and OVIS$^*$, respectively. 
Table~\ref{tab:pseudo} shows the attributes of the YTVIS21$^*$ and OVIS$^*$. The generation procedure is included in \texttt{{get\_pseudo\_data.py}}.

\section{Additional Results on VIS}
\label{app:vis}

\subsection{Datasets information}
YTVIS19\cite{masktrackrcnn} covers 40 object classes and contains 2,238/302 videos for training/validation. YTVIS21\cite{masktrackrcnn} retains the number of categories of YTVIS19 while expanding the datasets to 2,985/421 videos for training/validation and improving the instance annotation quality. OVIS\cite{ovis} has 25 object classes and contains 607/140 videos for training/validation. While the number of videos is less, each OVIS video includes more frames (69.4 frames on average) than YTVIS19 (27.6 frames) and YTVIS21 (30.2 frames). 
Moreover, OVIS samples typically involve more instances and severe occlusion and thus are more challenging.

\subsection{Without COCO Joint Training}
We provide results trained solely on video data (for a fair comparison with previous methods\cite{mask2formervis,crossvis}). 
As shown in Table~\ref{tab:wocjt}, CTVIS (ResNet-50 as the backbone)
trained without COCO data achieves 49.3 on AP on YTVIS21, close to
50.1 with COCO joint training. Meanwhile, CTVIS significantly outperforms previous methods under the same no-COCO setting.

\begin{table}[htbp]
  \centering
    \begin{tabular}{c|c|c}
    \toprule
    Methods & CJT   & \multicolumn{1}{l}{AP} \\
    \midrule
    CrossVIS \cite{crossvis} & \ding{53}     & 34.2 \\
    Mask2Former-VIS \cite{mask2formervis} & \ding{53}     & 40.6 \\
    CTVIS &  \ding{53}    & 49.3 \\
    CTVIS & $\checkmark$     & 50.1 \\
    \bottomrule
    \end{tabular}%
  \caption{Performance on YTVIS21 without using COCO joint training (CJT). We use the ResNet-50 as the backbone.}
  \label{tab:wocjt}%
\end{table}%

\subsection{Results on YTVIS22}

\begin{table}[htbp]
  \centering

    \begin{tabular}{c|c|ccc}
    \toprule
    \multicolumn{2}{c|}{Methods} & AP          & AP$^S$        & AP$^L$ \\
    \midrule
    \multirow{5}[2]{*}{\begin{sideways}ResNet-50\cite{resnet}\end{sideways}} & Mask2Former-VIS\cite{mask2formervis} & 35.4        & 40.7        & 30.2 \\
                & MinVIS\cite{minvis}      & 33          & 44.3        & 21.6 \\
                & VITA \cite{vita}       & 38.9        & 45.7        & 32 \\
                & IDOL \cite{idol}       & \underline{41.8}        & \underline{47.3}        & \underline{36.3} \\
                & \textbf{CTVIS (Ours)}     & \textbf{44.9} & \textbf{50.3} & \textbf{39.4} \\
    \midrule
    \multirow{5}[2]{*}{\begin{sideways}Swin-L\cite{swin}\end{sideways}} & Mask2Former-VIS\cite{mask2formervis} & 43.4        & 52.6        & 34.2 \\
                & MinVIS \cite{minvis}      & 44.3        & 55.5        & 33 \\
                & VITA \cite{vita}       & 49.3        & 57.7        & 41 \\
                & IDOL \cite{idol}       & \underline{52.3}        & \underline{60.7}        & \underline{44} \\
                & \textbf{CTVIS (Ours)}       & \textbf{53.8} & \textbf{61.2} & \textbf{46.4} \\
    \bottomrule
    \end{tabular}%

  \caption{Compare CTVIS with SOTA methods\cite{mask2formervis,vita,minvis,idol} on YTVIS22\cite{masktrackrcnn}. AP$^S$ and AP$^L$ denote the performance evaluated on short videos and long videos, respectively. AP is obtained by averaging AP$^S$ and AP$^L$ over classes.
  The best and second best are highlighted by \textbf{bold} and \underline{underlined} numbers, respectively.}
  \label{tab:ytvis22}%
\end{table}%

As shown in Table~\ref{tab:ytvis22}, we evaluate our CTVIS on YTVIS22 \cite{masktrackrcnn}, which shares the same training set with YTVIS21 and extends with 71 long videos for validation.  Because most methods do not report the results on YTVIS22,
we use the official source codes and model weights trained on YTVIS21 provided by the authors to measure
the average precision in this experiment. 
%With both ResNet-50 \cite{resnet} and Swin-L \cite{swin}, CTVIS outperforms other SOTA methods on all metrics. 
We observe that the performance improvement for long videos is significant as the CTVIS with ResNet-50 surpasses the previous SOTA offline method (VITA\cite{vita}) and online method (IDOL\cite{idol}) by 7.1 and 3.1 on AP$^L$, respectively. 
With the stronger backbone Swin-L, CTVIS outperforms the IDOL by 2.4 on AP$^L$, which suggests that CTVIS generalizes well to long complicated videos.

\subsection{Instance Embedding Visualization}
We visualize the learned instance embeddings by t-SNE\cite{tsne} in Figure~\ref{fig:visualize_query}. Each plot is for a video and the plot of the same color represents the identical video. The embeddings of the same instance (across different frames) is denoted by one particular color. As there are no annotations in the validation set, we select videos from the training set. For the VIS model\cite{idol} without consistent training (first row of Figure~\ref{fig:visualize_query}), instance embeddings are scattered. With consistent training, CTVIS learns more discriminative instance embeddings, which allows a robust tracking of instances in videos.

\begin{figure*}[t]
    \centering
    \includegraphics[width=1.0\textwidth]{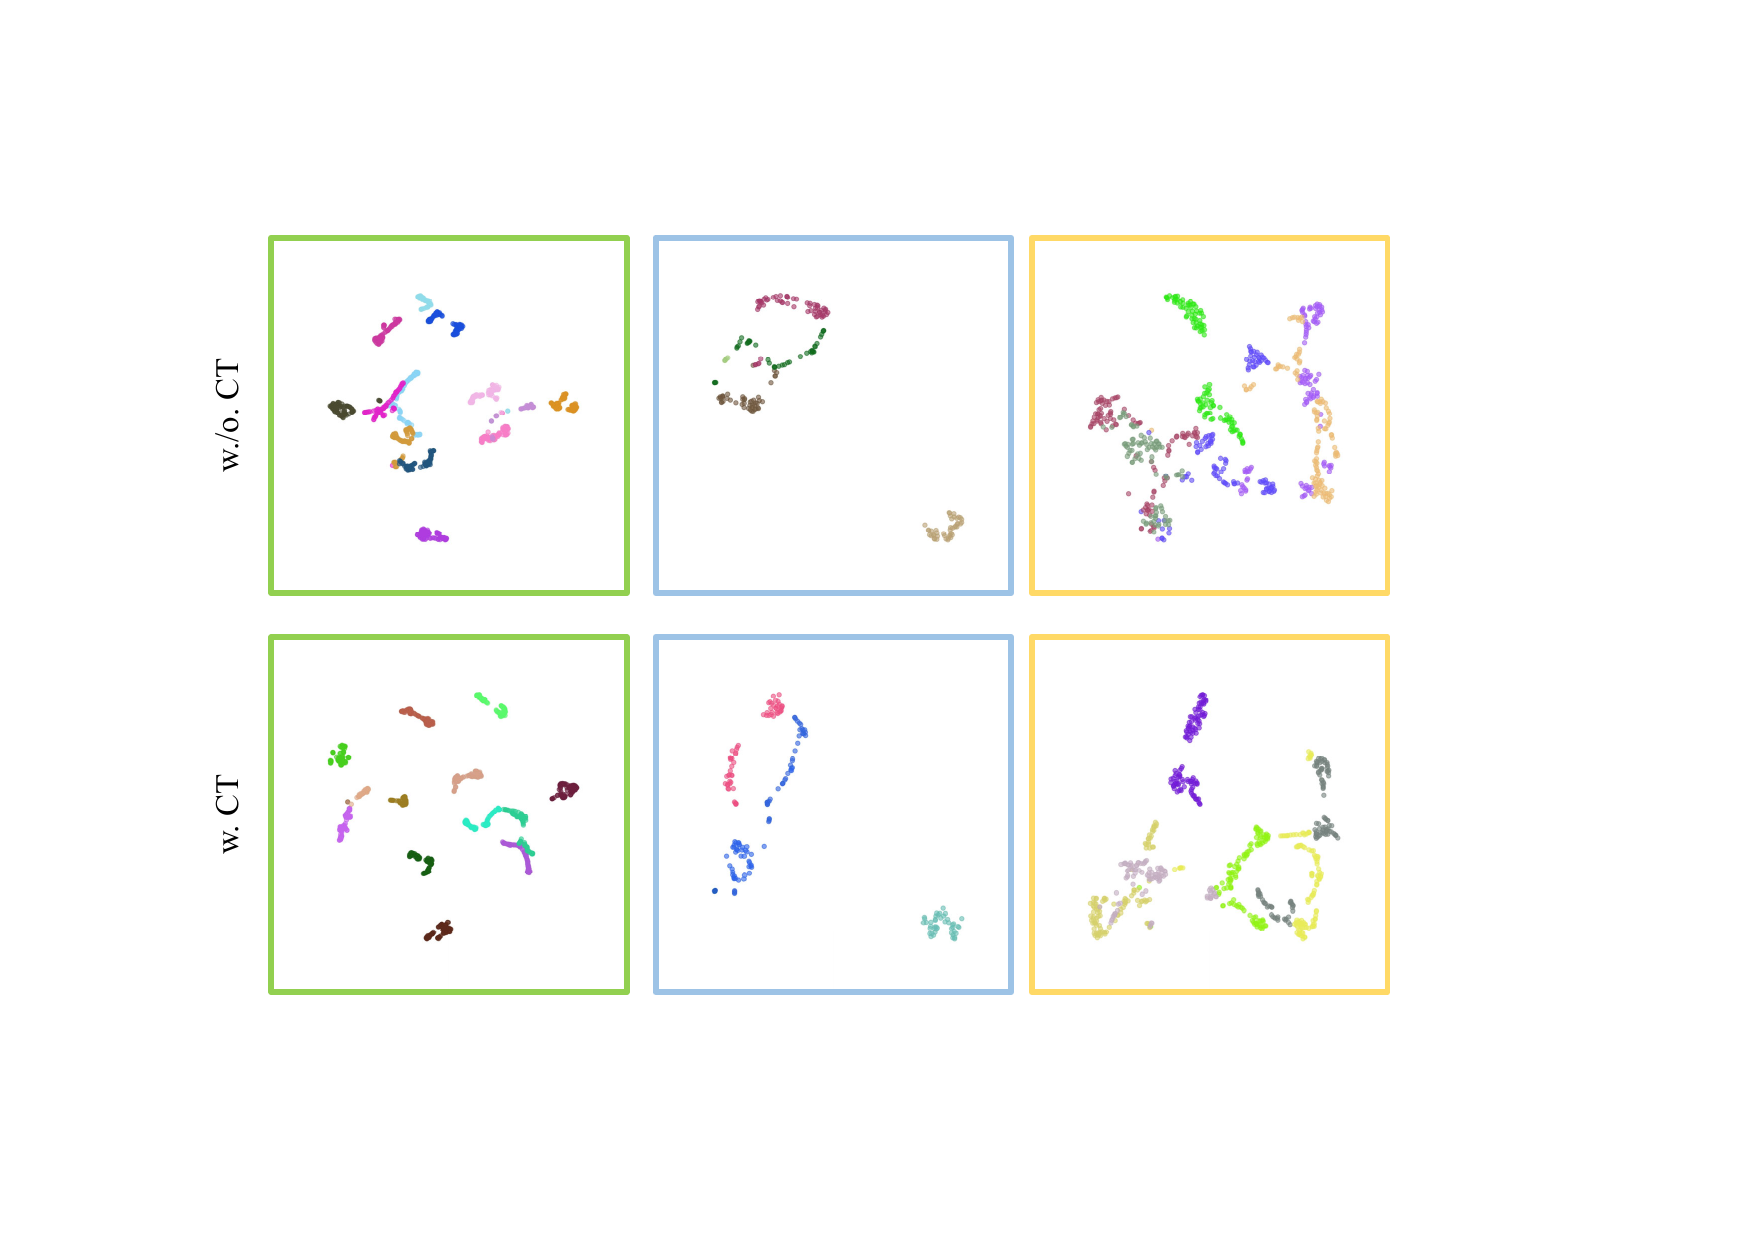}
    \caption{Visualization of instance embeddings without (w./o.) or with (w.) consistent training. Each plot is for a video, and plots of the same color represents an identical video. Within each plot, embeddings of the same instance (in different frames) take one particular color. Clearly, CTVIS enables the learning of more discriminative instance embeddings.
} 
    \label{fig:visualize_query}
\end{figure*}

\subsection{More Qualititative VIS Results}

\begin{figure*}[t]
    \centering
    \includegraphics[width=1.0\textwidth]{}
    \caption{Additional qualitative results of CTVIS with Swin-L\cite{swin} on the validation and testing set of OVIS\cite{ovis}. Each row represents a video. The same color denotes the same instance. Best viewed in color.} 
    \label{fig:visualize_vis}
\end{figure*}

Figure~\ref{fig:visualize_vis} gives additional results of CTVIS with Swin-L on the validation and testing sets of OVIS. 
CTVIS is capable of handling complex scenes that involve object occlusion, deformation, small-scale objects, and is able to obtain accurate segmentation results. 
We also provide a visualization video, please refer to \texttt{demo\_dance.mp4} for details.

\section{Extend to Video Panoptic Segmentation}
\label{app:vps}
Video panoptic segmentation (VPS) \cite{vps, vipseg} requires segmenting and tracking \textit{things} across video and segmenting stuff (\ie \textit{sky}, \textit{grass}) in each frame. In this appendix, we simply apply our proposed CTVIS to VPS.

\begin{table*}[htbp]
  \centering
    \begin{tabular}{c|c|cccc}
    \toprule
    Methods     & Backbone    & VPQ         & VPQ$^{Th}$    & VPQ$^{St}$    & STQ \\
    \midrule
    VPSNet\cite{vps}      & ResNet-50   & 14          & 14          & 14.2        & 20.8 \\
    VPSNet-SiamTrack\cite{vps_siam} & ResNet-50   & 17.2        & 17.3        & 17.3        & 21.1 \\
    VIP-Deeplab\cite{vip_deeplab} & ResNet-50   & 16          & 12.3        & 18.2        & 22 \\
    Clip-PanoFCN\cite{vipseg} & ResNet-50   & 22.9        & 25          & 20.8        & 31.5 \\
    TarVIS $^*$ \cite{tarvis}      & ResNet-50   & 33.5        & \textbf{39.2}        & 28.5        & 43.1 \\
    \textbf{CTVIS (Ours)}       & ResNet-50   & \textbf{37.5}            & 36.8             & \textbf{38.2}       & \textbf{44.7} \\
    \midrule
    TarVIS $^*$ \cite{tarvis}      & Swin-L      & 48          & \textbf{58.2}        & 39          & 52.9 \\
    \textbf{CTVIS (Ours)}       & Swin-L      & \textbf{49.5}        & 48.9        & \textbf{49.9}        & \textbf{56.4}  \\
    \bottomrule
    \end{tabular}%
  \caption{Compare CTVIS with SOTA VPS methods on VIPseg. $*$ indicates that TarVIS introduces other video segmentation datasets to train a unified model.}
  \label{tab:vipseg}%
\end{table*}%

\subsection{Results on VIPSeg}
We select the VIPSeg as the dataset, which is a challenging dataset with 2,806/343 in-the-wild videos for training/validation. It contains 124 semantic classes (58 \textit{thing} and 66 \textit{stuff} classes). 
Following prior works \cite{vipseg, tarvis}, we use the VPQ, VPQ$^{Th}$, VPQ$^{St}$ and STQ as the evaluated metrics. We evaluate CTVIS with ResNet-50 and Swin-L as backbones, respectively. 

As shown in Table~\ref{tab:vipseg}, CTVIS is very competitive in comparison with SOTA models \cite{vps,vps_siam,vip_deeplab,vipseg,tarvis} proposed for VIPSeg. Please note that TarVIS\cite{tarvis} also takes Mask2Former\cite{mask2former} as the base segmentation model and trains on multiple segmentation datasets\cite{masktrackrcnn,ovis,vipseg}. In comparison, CTVIS is simply trained on the VIPSeg dataset, which outperforms TarVIS in all metrics except for VPQ$^{Th}$. Specifically, with the Swin-L backbone, CTVIS outperforms TarVIS by 3.5 in STQ, which is the most important metric.

\subsection{Visualization Results}

\begin{figure*}[t]
    \centering
    \includegraphics[width=1.0\textwidth]{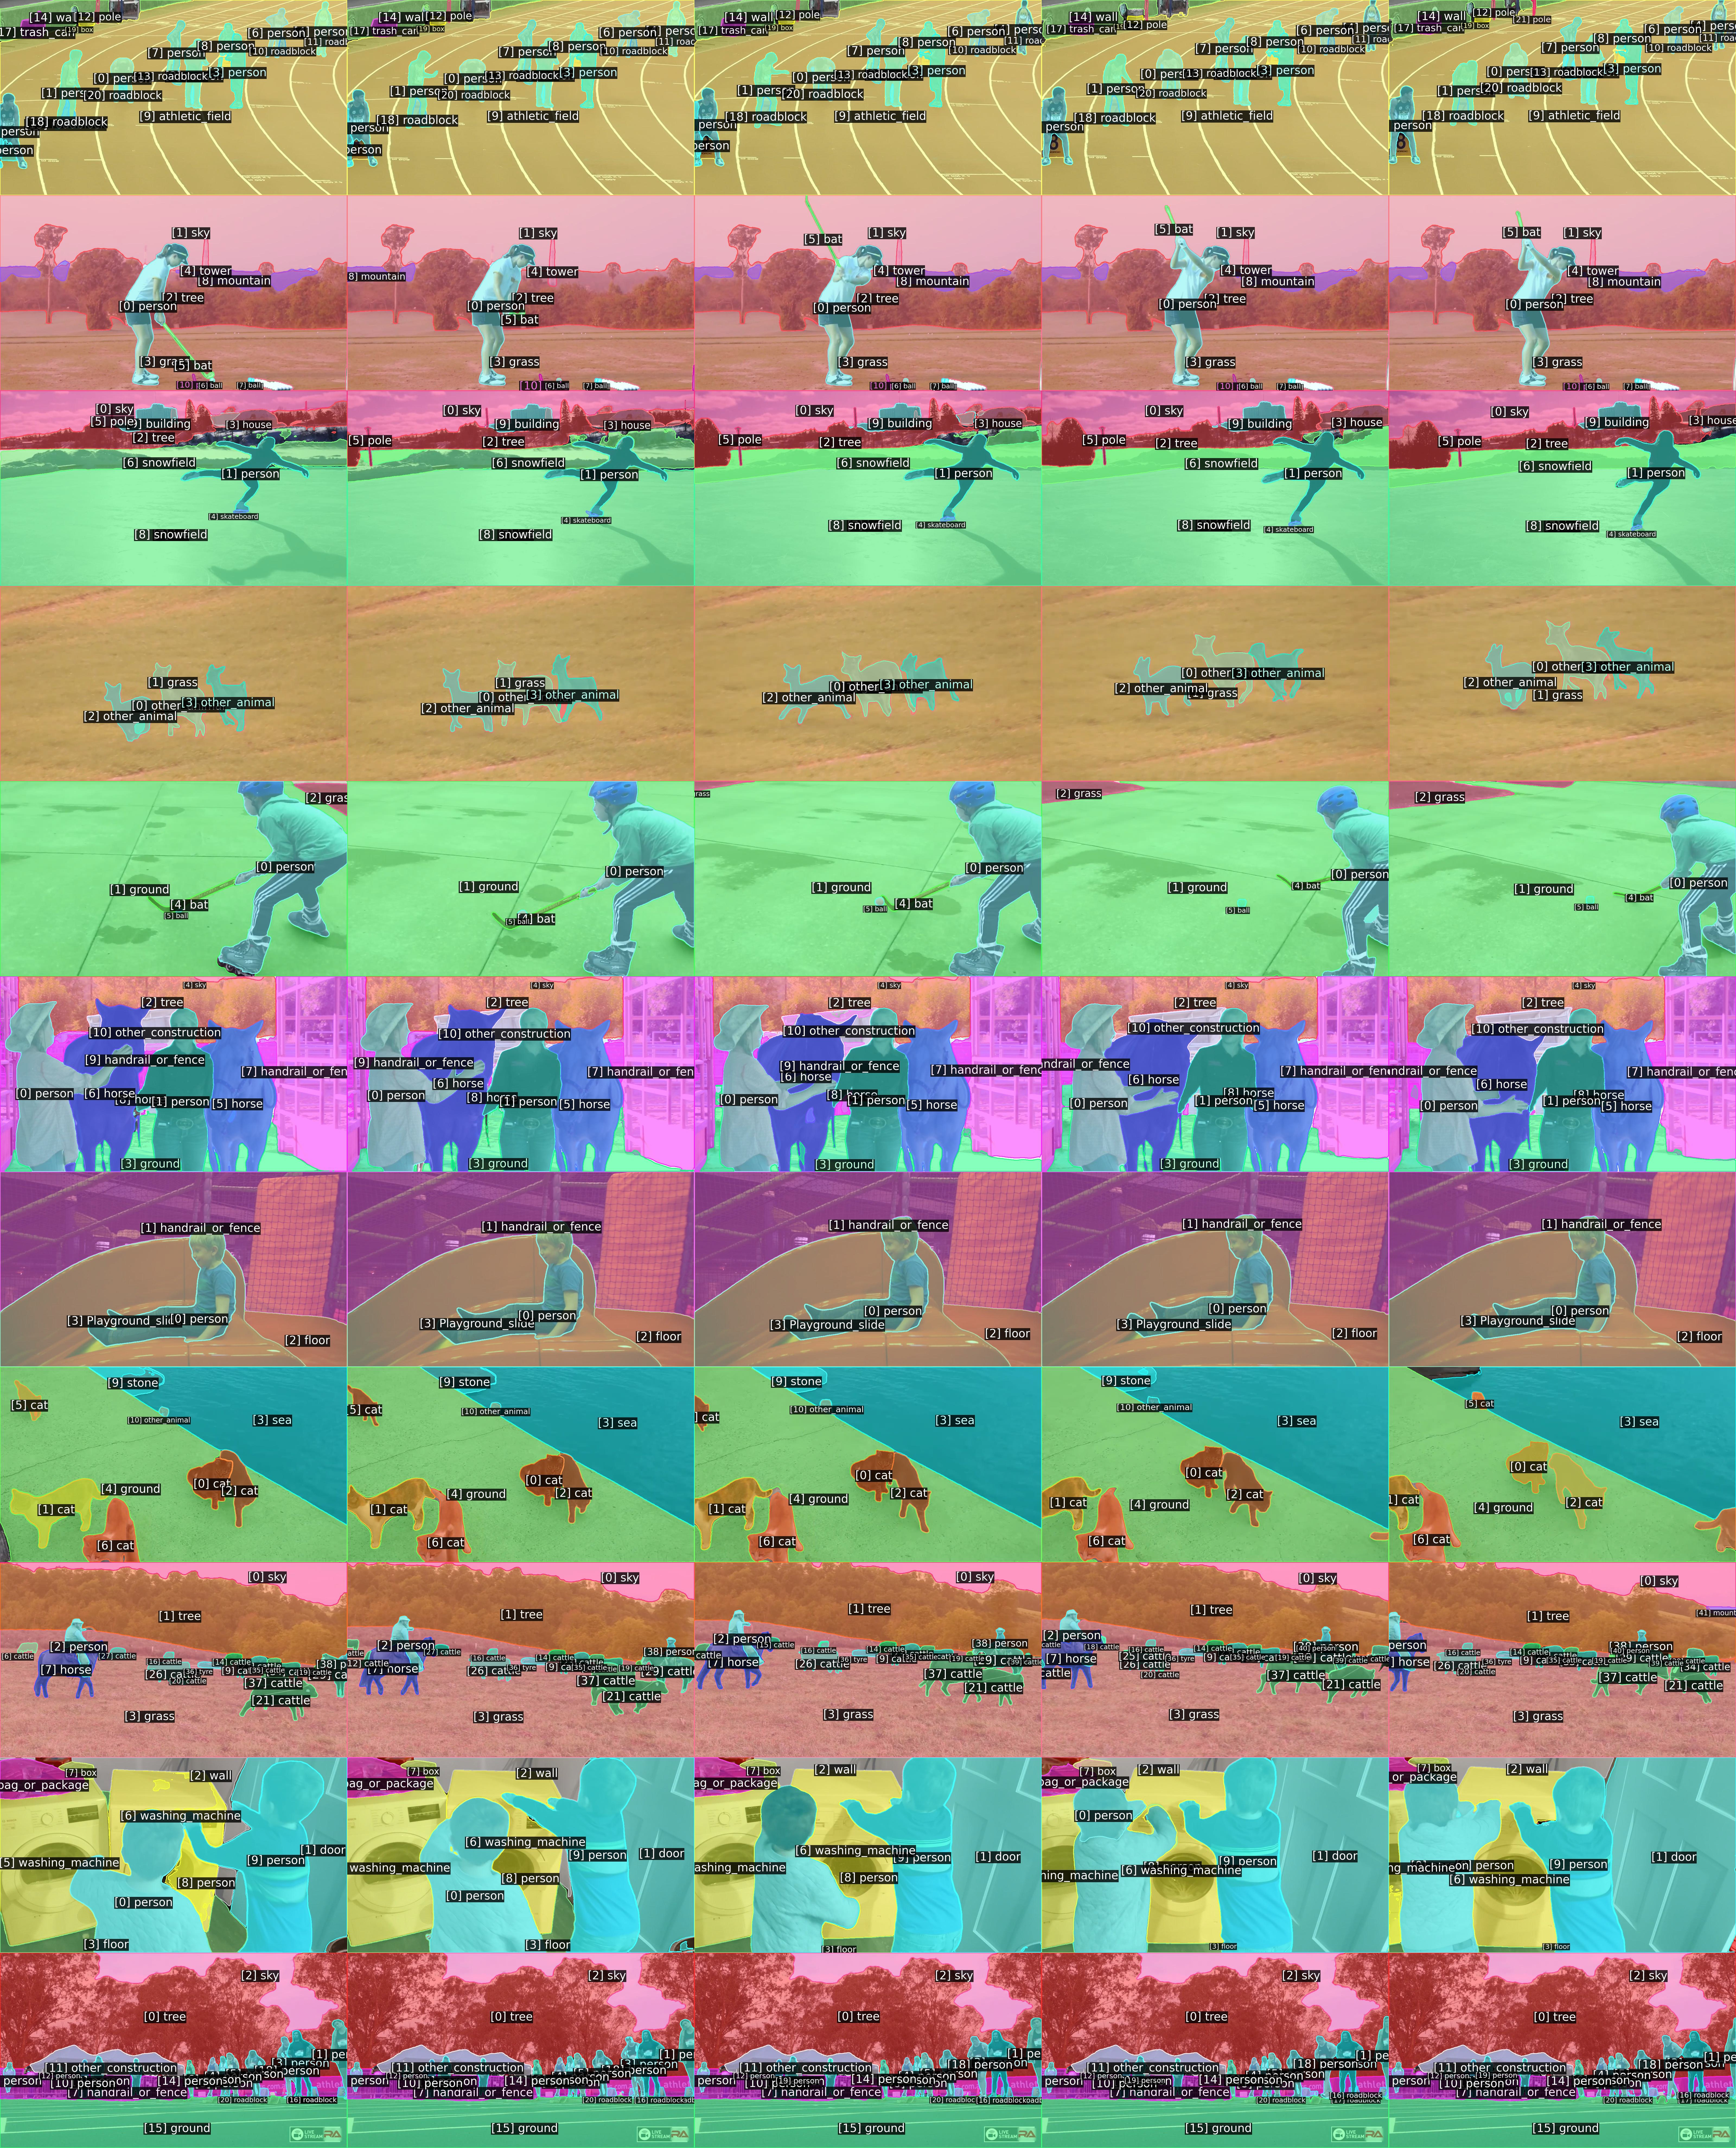}
    \caption{Qualitative results of CTVIS with Swin-L\cite{swin} on the testing set of VIPSeg \cite{vipseg}. Each row represents a video. The same color represents the same instance. Best viewed in color.} 
    \label{fig:visualize_vps}
\end{figure*} 

We visualize the qualitative results of CTVIS with ResNet-50 on the testing set of VIPSeg\cite{vipseg} in Figure~\ref{fig:visualize_vps}, where CTVIS offers superior segmentation results even for complex scenes.
